# Supplementary material for: Spontaneous frequency shift and phase delay of coupled terahertz radiations mediated by the Josephson plasmon in a cuprate superconductor
Source: arXiv:2109.08845 source file (2022-04-20)
Supplement: Supplementary file 1 [file SM_20220311.pdf]

# Supplementary Materials for
# "Spontaneous frequency shift and phase delay of coupled terahertz radiations mediated by the Josephson plasmon in a cuprate superconductor ."

Ryota Kobayashi,[1, *] Ken Hayama,[1, *] Shuma Fujita,[1] Manabu Tsujimoto,[2] and Itsuhiro Kakeya[1, †]

[1]*Department of Electronic Science and Engineering, Kyoto University, Kyotodaigaku Katsura, Nishikyo, Kyoto 615-8510, Japan*
[2]*Research Center for Emerging Computing Technologies, National Institute of Advanced Industrial Science and Technology (AIST), Central2, 1-1-1 Umezono, Tsukuba, Ibaraki 305-8568, Japan.* [‡]

(Dated: March 12, 2022)

## Si. BASIC PROPERTIES OF INDIVIDUAL MESAS

Geometries, superconducting transition temperature $T_c$ characterizing mesas B, C, and E are listed in Table SI. The length and thickness of the mesas are designed to be the same as 350 and 80 $\mu$m. Figure S1 shows current-voltage-emission characteristics for mesas B, C, and E. Dominant high-bias emission and weak low-bias emission were found [1]. The high-bias emission was found in all mesas and the low-bias emission was found in mesas C and E. The high bias emission is pronounced below 35, 25, and 45 K for mesas B, C, E, respectively. Thus, subsequent discussion to compare individual and simultaneous emissions is done for data acquired at 30 K.

Temperature dependence of the radiation intensity for individual biasing are shown in Fig. S2. The intensity maxima in B and E are found at 30 and 36 K, respectively. Comparing the intensity at 30 K, where simultaneous bias data were taken, with the data at higher temperatures, E can increase by more than 10 % with a temperature rise of about 6 K, but B decreases by more than that, so that the sum of intensities is smaller than that at 30 K. For these reasons, we can conclude that the radiation intensity in simultaneous bias is not due to the temperature increase added to the superposition of the individual radiations.

TABLE SI. Properties of individual mesas B, C, and E. In upper rows, basic superconducting and emission properties are listed. In middle rows, maximum detection voltages of the bolometer $P_{max}$ and bias current and voltages where $P_{max}$ is obtained at 30 K are listed. In lower rows, Stokes polarization parameters $\mathbf{S} = (S_0, S_1, S_2, S_3) = S_0(1, \tilde{S_1}, \tilde{S_2}, \tilde{S_3})$ and $DoP = \sqrt{\tilde{S_1}^2 + \tilde{S_2}^2 + \tilde{S_3}^2}$ at frequencies giving the maximum $S_0$ are listed.

| | B | C | E |
|---|---|---|---|
| $T_c$ | 78.5 | 79.3 | 78.3 |
| Mesa width ($\mu$m) | 66.8 | 68.2 | 66.1 |
| $P_{max}$ (mV) | 0.418 | 0.215 | 0.468 |
| Bias current (mA) | 21.9 | 33.8 | 21.7 |
| Bias voltage (V) | 0.983 | 1.01 | 0.963 |

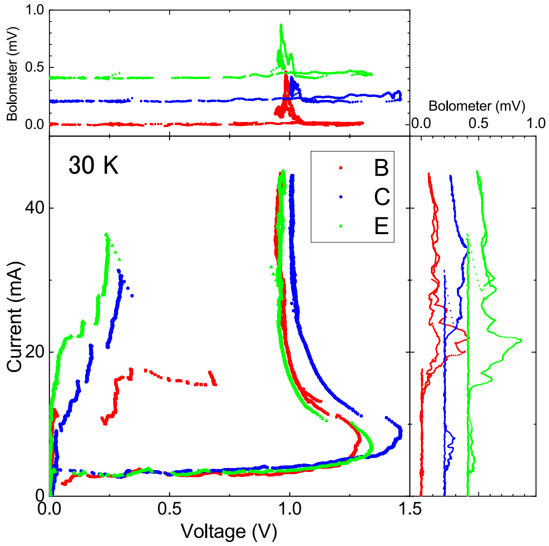


FIG. S1. Current-voltage characteristics (main) and bolometer responses as a function of either current (right) or voltage (upper) for mesas B (black), C (red), and E (blue). The bolometer responses are shifted for clarity. Higher bolometer responses correspond to the case for bias swept-down.

## Sii. POLARIZATION DATA ACQUISITION

The voltage/current dependences of SPPs were extracted from $I - V - E$ curves at varied QWP angle $\theta$ of the system shown in Ref. [2]. First, we obtained $I - V - E$ data at every fixed $\theta$ for several $I - V$ rounds, where $\theta$ was changed from 0 to 360 degrees with a step of 9 or 18 degrees. Second, a polar plot of the transmission intensities was made to pick up $E$-values within a certain

* These authors contributed equally.
† kakeya@kuee.kyoto-u.ac.jp; Corresponding author
‡ Faculty of Pure and Applied Sciences, University of Tsukuba, 1-1-1 Tennodai, Tsukuba, Ibaraki 305-8573, Japan

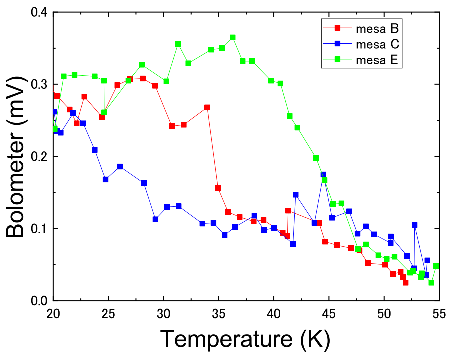


FIG. S2. Temperature dependence of the maximum radiation intensity for individual B, C, and E.

TABLE SII. (a-c) Derived stokes polarization parameters at given individual and simultaneous bias conditions.

| | | Bias | $S_0$ | $\tilde{S}_1$ | $\tilde{S}_2$ | $\tilde{S}_3$ |
|---|---|---|---|---|---|---|
| (a) | B | 0.918 V | 0.341 | 0.912 | 0.245 | -0.328 |
| | E | 0.917 V | 0.362 | 0.819 | 0.041 | 0.571 |
| | B‖E | 0.921 V | 0.696 | 0.953 | 0.204 | 0.219 |
| (b) | B | 0.974 V | 0.530 | 0.728 | 0.513 | -0.453 |
| | E | 0.984 V | 0.471 | 0.722 | -0.104 | 0.683 |
| | B‖E | 0.974 V | 0.528 | 0.699 | -0.167 | 0.694 |
| (c) | B | 30 mA | 0.341 | 0.912 | 0.245 | -0.328 |
| | E | 30 mA | 0.517 | 0.767 | 0.050 | 0.638 |
| | B−E | 30 mA | 1.079 | 0.862 | 0.062 | 0.501 |

$I-V$ window (e.g., 1 mA × 0.05 V ) for $\theta$s. Here, E-data points which apparently deviates from the two-fold rotational (C2) symmetry were removed. Then, SPPs were obtained by fitting

$$I(\theta) = \frac{1}{2}\left(S_0 + S_1 \cos^2 2\theta + S_2 \cos 2\theta \sin 2\theta + S_3 \sin 2\theta\right), \tag{S1}$$

to the polar plot. The obtained values compose SPPs at the bias of the center of the I-V window.

For comparisons among different mesas and different connections, normalized SPPs $(1, \tilde{S}_1, \tilde{S}_2, \tilde{S}_3)$, where $\tilde{S}_i = S_i/S_0$ $(i = 1, 2, 3)$ are useful and the degree of polarization $DoP$ is written as

$$DoP = \frac{\sqrt{{S_1}^2 + {S_2}^2 + {S_3}^2}}{S_0} = \sqrt{\tilde{S}_1^2 + \tilde{S}_2^2 + \tilde{S}_3^2}. \tag{S2}$$

Examples of obtained SPPs used to estimate $\alpha$ and $\beta$ according to Sec. III.C.1 are listed in Table SII.

## Siii. CORRECTION FUNCTION FOR TWO-FOLD ASYMMETRY

Since the QWP used in this work consists of thin metallic plates held by a pair of pillars [3], a possible local

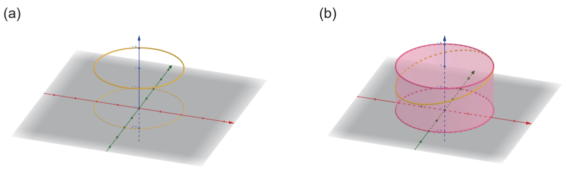


FIG. S3. Schematic representations of the correction function $C(\theta)$. (a) Homogeneous loss case with $C(\theta) = 1$. (b) Assume that the observed transmission intensity is a result of a linearly-dependent spatial loss (of the QWP). Observed intensity corresponds to the red circle with respect to real incident intensity represented by the yellow ellipse with $C(\theta) = 1 + 0.25\sin(\theta + 1) - 0.25$.

deformation of the plates results in asymmetric transmission through the QWP. This is pronounced when the THz beam is not centered at the QWP. To obtain reliable SPPs, we introduce a correction function $C(\theta)$, Eq. (2) in the main text. $C(\theta)$ is found from $2\pi$ periodic functions with respect to $\theta$ and restore the loss of QWP due to the deformation. Thus $\max_{0\le\theta<2\pi}\{C(\theta)\} = 1$ is satisfied as shown in Fig. S3.

## Siv. TRANSFORMATION FROM STOKES POLARIZATION PARAMETERS TO ELECTRIC VECTOR

Consider a completely polarized electromagnetic wave whose electric field in the plane perpendicular to the propagation vector given by

$$\boldsymbol{E}(t) = \begin{pmatrix} E_x \exp[i\omega t] \\ E_y \exp[i(\omega t + \delta_{xy})] \end{pmatrix}, \tag{S3}$$

where the observation plane is taken at $z = 0$ and $\omega$ is the angular frequency of the wave. The polarization of this electromagnetic wave is represented by a set of SPPs

$$\begin{pmatrix} S_0 \\ S_1 \\ S_2 \\ S_3 \end{pmatrix} = \begin{pmatrix} E_x^2 + E_y^2 \\ E_x^2 - E_y^2 \\ 2E_xE_y \cos\delta_{xy} \\ 2E_xE_y \sin\delta_{xy} \end{pmatrix}. \tag{S4}$$

The parameters of the electric field is oppositely obtained by the SPPs as

$$E_x = \sqrt{\frac{S_0 + S_1}{2}}, \tag{S5}$$

$$E_y = \sqrt{\frac{S_0 - S_1}{2}}, \tag{S6}$$

$$\delta_{xy} = \arctan\frac{S_3}{S_2}, \tag{S7}$$

which are used to obtain complex coefficients of $\alpha$ and $\beta$ with Eq. (5) in the main text.

[1] I. Kakeya and H. Wang, Superconductor Science and Technology **29**, 073001 (2016).
[2] M. Tsujimoto, S. Fujita, G. Kuwano, K. Maeda, A. Elarabi, J. Hawecker, J. Tignon, J. Mangeney, S. Dhillon, and I. Kakeya, Physical Review Applied **13**, 051001 (2020).
[3] M. Nagai, N. Mukai, Y. Minowa, M. Ashida, T. Suzuki, J. Takayanagi, and H. Ohtake, Optics Express **23**, 4641 (2015).
